# Supplementary material for: Stability Guarantees for Feature Attributions with Multiplicative Smoothing
Source: arXiv:2307.05902 source file (2023-10-26)
Supplement: Supplementary file 1 [file selective_masking.tex]

Observe that the definition of stability quantifies over masks \(\alpha \succeq \varphi(x)\).
Thus, any such \(\alpha\) can be split as \(\alpha = \varphi(x) + \delta\), where \(\varphi(x)\) and \(\delta\) are binary vectors with disjoint ones entries.
This suggests that perturbations (i.e. smoothing) should only apply to the non-explanatory features, and so motivates us to construct an explainable model \(\angles{f_\mu, \varphi}\), where \(\mu \in \{0,1\}^n\) is a parameter that is dependent on \(\varphi\).
In particular, we take \(\mu = \varphi(x)\) to mean which coordinates to smooth: let \(\mu_i = 0\) mean that the \(i\)th coordinate should be smoothed, and let \(\mu_i = 1\) mean that the \(i\)th coordinate should \emph{not} be smoothed.
This then exactly corresponds to smoothing only the non-explanatory features.
Evaluating \(\angles{f_\mu, \varphi}(x)\) on some \(x \in \mcal{X}\) therefore consists of first finding \(\mu = \varphi(x)\), and then evaluating \(f_\mu (x)\).
We use \(\lor\) to mean the coordinate-wise logical OR on binary vectors, and present the following.

\begin{theorem}[\mus{} with Selective Masking] \label{thm:mus-selective}
    Let \(\mcal{D}\) be as in Theorem~\ref{thm:mus} and fix any \(\mu \in \{0,1\}^n\).
    Consider any \(h : \mcal{X} \to [0,1]\) and define \(g_\mu : \mcal{X} \times \{0,1\}^n \to [0,1]\) as
    \begin{align*}
        g_\mu (x, \alpha) = \expval{s \sim \mcal{D}} h(x \odot \tilde{\alpha}),
        \qquad
        \tilde{\alpha} = \mu \lor (\alpha \odot s)
    \end{align*}
    Then the function is \(g_\mu (x, \cdot) : \mcal{X} \to [0,1]\) is \(\lambda\)-Lipschitz in the \(\ell^1\) norm for all \(x \in \mcal{X}\).
\end{theorem}
\begin{proof}
Similar to the proof of Theorem~\ref{thm:mus}, fix any \(s \sim \mcal{D}\), consider any \(x \in \mcal{X}\), let \(\alpha, \alpha' \in \{0,1\}^n\), and define \(\delta = \alpha - \alpha'\).
Observe that if \(\mu_i = 1\), then we have \(\tilde{\alpha}_i = \tilde{\alpha}_i ' = 1\).
On the other hand if \(\mu_i = 0\), then \(\tilde{\alpha}_i \neq \tilde{\alpha}_i '\) exactly when \(\abs{\delta}_i = 1\) and \(s_i = 1\).
Since \(s_i \sim \mcal{B}(\lambda)\), this means that
\begin{align*}
    \mrm{Pr}[\tilde{\alpha}_i \neq \tilde{\alpha}_i ']
    = (1 - \mu_i) \lambda \abs{\delta_i}
    \leq \lambda \abs{\delta_i},
\end{align*}
and the rest of the proof is identical to that of Theorem~\ref{thm:mus} starting from the union bound step.
\end{proof}

The case of \(\mu = \mbf{0}\) makes the above result identical to Theorem~\ref{thm:mus}.
We will define such a smoothed classifier with the mapping \(f_\mu (z) = g_\mu (z, \mbf{1})\).
We next show in Proposition~\ref{prop:mus-selective-equivalence} that selective masking preserves masking-equivalence under the assumption that \(\alpha \succeq \mu\), which always holds since for stability we only analyze the masks \(\alpha \succeq \mu = \varphi(x)\).

\begin{proposition}
\label{prop:mus-selective-equivalence}
    Take \(g_\mu\) as in Theorem~\ref{thm:mus-selective}.
    If \(\alpha \succeq \mu\), then
    \(g_\mu (x, \alpha) = g_\mu (x \odot \alpha, \mbf{1})\) for all \(x \in \mcal{X}\).
\end{proposition}
\begin{proof}
Observe that if \(\alpha \succeq \mu\), then \(x \odot \alpha \odot \mu = x \odot \mu\).
Thus:
\begin{align*}
    g_\mu (x, \alpha)
        &= \expval{s \sim \mcal{D}}
            h(x \odot (\mu \lor (\alpha \odot s)))
            \tag{\(\tilde{\alpha} = \mu \lor (\alpha \odot s)\)}
            \\
        &= \expval{s \sim \mcal{D}}
            h ((x \odot \mu) \lor (x \odot \alpha \odot s)) \\
        &= \expval{s \sim \mcal{D}}
            h ((x \odot \alpha \odot \mu) \lor (x \odot \alpha \odot s))
            \tag{\(\alpha \succeq \mu\)} \\
        &= \expval{s \sim \mcal{D}}
            h((x \odot \alpha) \odot (\mu \lor s)) \\
        &= g_\mu (x \odot \alpha, \mbf{1})
            \tag{\(\mu \lor s = \mu \lor (\mbf{1} \odot s)\)}
\end{align*}
\end{proof}

Although the condition of \(\alpha \succeq \mu\) makes this result more restrictive than the earlier version of masking equivalence in~\eqref{eq:masking-equivalence}, it nevertheless give us a way to check for certified stability.

\begin{theorem}[Stability with Selective Masking] \label{thm:mus-selective-stability}
Let \(g_\mu\) be as in Theorem~\ref{thm:mus-selective} and consider any explanation method \(\varphi\).
Let \(f_\mu (z) = g_\mu (z, \mbf{1})\) where \(\mu \in \{0,1\}^n\) is a parameter, and define the explainable model \(\angles{f_\mu, \varphi}\).
Consider any \(x \in \mcal{X}\) and fix \(\mu = \varphi(x)\).
Then for any \(\alpha \succeq \varphi(x)\) we have:
\begin{align*}
    &\norm{\alpha - \varphi(x)}_1
        \leq \frac{g_A (x, \varphi(x)) - g_B (x, \varphi(x))}{2 \lambda}
    &&\implies
        f_\mu (x \odot \alpha) \cong f_\mu (x \odot \varphi(x)) \\
    &\norm{\mbf{1} - \alpha}_1
        \leq \frac{g_A (x, \mbf{1}) - g_B (x, \mbf{1})}{2 \lambda}
    &&\implies f_\mu (x) \cong f_\mu (x \odot \alpha)
\end{align*}
where \(g_A, g_B\) are the first and second largest logits of \(g_\mu\) analogously defined as in~\eqref{eq:logit-gap}.
\end{theorem}
\begin{proof}
Fix \(x \in \mcal{X}\) and consider any \(\alpha \succeq \varphi(x)\).
Then by Proposition~\ref{prop:mus-selective-equivalence} we have:
\begin{align*}
    f(x \odot \alpha) = g(x \odot \alpha, \mbf{1})
    = g(x, \alpha).
\end{align*}
The rest of the incremental stability proof is identical to that of Theorem~\ref{thm:stability}, where for decremental stability note that \(\mbf{1} \succeq \varphi(x)\) allows us to trivially apply masking equivalence.
\end{proof}
